# Supplementary material for: Multimodal Pretrained Models for Verifiable Sequential Decision-Making: Planning, Grounding, and Perception
Source: arXiv:2308.05295 source file (2024-06-17)
Supplement: Supplementary file 1 [file A-appendix.tex]

\newpage
\appendix

% \begin{figure*}[t]
\onecolumn

% \begin{figure}
%     \centering
%     \input{figures/0_draft_and_old_figures/cross_road1_old}
%     \input{figures/0_draft_and_old_figures/cross_road2_simple}
%     \caption{Caption}
%     \label{fig:my_label}
% \end{figure}

\section{Additional Preliminaries}
\subsection{Product Automata}
Let
$\Aut[model] \coloneqq
\langle
    \AutStates[model],
    \AutSymbsIn[model],
    \AutSymbsOut[model],
    \AutTransFunc[model],
    \AutLabelFunc[model]
\rangle$ be a model and let
$\Aut[controller] \coloneqq
\langle
    \AutStates,
    \AutSymbsIn,
    \AutSymbsOut,
    \Autstate_0,
    \AutTransFunc,
    \AutLabelFunc
\rangle$ be a controller, 
we define the \emph{product automaton} as an \gls{aut}
$\Aut[product] =
\Aut[model] \otimes \Aut[controller] \coloneqq
\langle
    \AutStates[product],
    % \AutSymbsIn[product],
    \AutTransFunc[product],
    \Autstate[product-init],
    \AutLabelFunc[product]
\rangle
$
as follows:
\begin{align*}
\AutStates[product] &\coloneqq \AutStates[model] \times \AutStates
\\
% \AutSymbsIn[product] &\coloneqq \AutSymbsIn = 2^{\AutProps}
% \\
\AutTransFunc[product]( (p, q))
&\coloneqq
\left\{
    (p', q') \in \AutStates[product] \middle|
    \AutTransFunc(q, c, q') = 1
    \land
    \AutTransFunc[model](p, \Autsymbout, p') = 1
\right\}
\\
&\text{where } \Autsymbout = \AutLabelFunc(q, \Autsymbin, q') \text{ and } c = \AutLabelFunc[model](p)
\\
\Autstate[product-init] &\coloneqq (p, \Autstate[init]) \quad \text{where $p$ can be any state in }\Aut[model]
\\
\AutLabelFunc[product]((p, q)) &\coloneqq \AutLabelFunc[model](p) \cup \AutLabelFunc(q, \AutLabelFunc[model](p), q') \quad \text{where } q' \in \AutStates \text{ and } \AutTransFunc(q, \AutLabelFunc[model](p), q') = 1.
\end{align*}
The trajectories from $\Aut[product]$ are in the form $(2^{ \AutProps[model] \cup \overline{P} })^{*}$, i.e. \( \psi_0, \psi_1, \psi_2 \ldots \) where $\psi_i = \AutLabelFunc[product](q_i, p_i)$.

\section{Additional Grammar Rules}

\begin{table}[ht]
\centering
\begin{tabular}{m{0.3\linewidth} m{0.35\linewidth} m{0.3\linewidth}}
\hline
Natural Language Grammar & Formal Representation & Example\\
\hline
\vspace{0.2cm}
VP$_1$ \textbf{and} VP$_2$ & VP$_1 \land$ VP$_2$ & [green light] [and] [no car] \\ 
VP$_1$ \textbf{or} VP$_2$ & VP$_1 \vee$ VP$_2$ & [traffic light] [or] [crosswalk] \\
\textbf{no/not} VP$_1$ & $\neg$ VP$_1$ & [no] [car] \\
\hline

\shortstack{VP$_1$ \textbf{[step number j]}} & \vspace{0.2cm}\input{figures/rules/direct_trans.tex} & [go to step]  [1]\\
\hline

\shortstack{ \textbf{if} $\:$ VP$_1$, $\:$ VP$_2$. \\ VP$_2$ $\:$ \textbf{if} $\:$ VP$_1$} &
\vspace{0.2cm}\input{figures/rules/cond.tex} & [if] [green light], [cross] \\

\shortstack{ \textbf{if} VP$_1$, VP$_2.\:$ \textbf{if} VP$_3$, VP$_4.$} &
\vspace{0.2cm}\input{figures/rules/cond_multi.tex} & [if] [car], [stay]. [if] [no car], [cross].\\

\shortstack{\textbf{if} VP$_1$, VP$_{2}$ \textbf{else} VP$_{3}.$ \\ 
$\text{VP}_{2}$ \textbf{if} VP$_1$, \textbf{else} VP$_{3}$} &
\vspace{0.2cm}\input{figures/rules/cond_merge.tex} & [if] [car], [stay], [else] [cross].\\
\hline

\shortstack{ \textbf{wait} VP$_1$ VP$_2$ \\ VP$_2$ \textbf{after} VP$_1$ } &
\vspace{0.2cm} \input{figures/rules/self_trans.tex} & [wait] [green light] [cross]\\

\shortstack{ VP$_2$ \textbf{until} VP$_1$} &
 \input{figures/rules/self_trans_until.tex} & [not cross] [until] [green light]\\
\hline

\shortstack{VP$_1$} &
\vspace{0.2cm} \input{figures/rules/default_trans.tex} & [cross road]\\
\hline

\end{tabular}
\caption{
    Rules to convert natural language grammar to formal representations (propositions or FSA transitions). The keywords that define the grammar are in bold.
}
\label{tab: grammar1}
\end{table}

\section{Proofs}
\paragraph{Proof of Theorem \ref{thm: prob}}

\begin{proof}
    Let $ e_1 = $ "the condition is (actually) true," $ e_2 = $ "the condition is evaluated to be true," $ e_3 =$ "the condition is evaluated to be false," and $ e_u = $ "the condition is evaluated to be \UNC{}." The probability of Assumption 1 being held is
    \begin{equation}
        \begin{split}
            \mathbb{P}[\mathcal{A}_1=true] &= \mathbb{P}[\neg e_u \implies (e_2 \land e_1) \vee (e_3 \land \neg e_1)]\\
            & = \mathbb{P}[  e_u \vee (e_2 \land e_1) \vee (e_3 \land \neg e_1) ].
        \end{split}
    \end{equation}
    Since $e_2$, $e_3$, and $e_u$ are mutually exclusive events, we can write the probability as
    \begin{equation}
        \begin{split}
            \mathbb{P}[\mathcal{A}_1=true] &= \mathbb{P}[ e_u ] + \mathbb{P}[e_2 \land e_1] + \mathbb{P} [e_3 \land \neg e_1 ] \\
            & = \mathbb{P}[ e_u ] + \mathbb{P}[ e_1 | e_2 ]\cdot \mathbb{P}[ e_2 ] + \mathbb{P}[ \neg e_1 | e_3 ]\cdot \mathbb{P}[ e_3 ].
        \end{split}
    \end{equation}
    Based on the definition, $\mathbf{p}_t = \mathbb{P}[ e_1 | e_2 ]$ and $\mathbf{p}_f = \mathbb{P}[ \neg e_1 | e_3 ]$. And we know that $\mathbb{P}[ e_2 ] + \mathbb{P}[ e_3 ] + \mathbb{P}[ e_u ] = 1$. Hence
    \begin{equation}
        \begin{split}
            \mathbb{P}[\mathcal{A}_1=true] &= \mathbb{P}[ e_u ] + \mathbb{P}[ e_1 | e_2 ]\cdot \mathbb{P}[ e_2 ] + \mathbb{P}[ \neg e_1 | e_3 ]\cdot \mathbb{P}[ e_3 ] \\ 
            &= \mathbb{P}[ e_u ] + \mathbf{p}_t \cdot \mathbb{P}[ e_2 ] + \mathbf{p}_f \cdot \mathbb{P}[ e_3 ] \\
            & \ge \min (\mathbf{p}_t, \mathbf{p}_f) \cdot \mathbb{P}[ e_u ] + \min (\mathbf{p}_t, \mathbf{p}_f) \cdot \mathbb{P}[ e_2 ] + \min (\mathbf{p}_t, \mathbf{p}_f) \cdot \mathbb{P}[ e_3 ] \\
            & = \min (\mathbf{p}_t, \mathbf{p}_f) \cdot (\mathbb{P}[ e_u ] + \mathbb{P}[ e_2 ] + \mathbb{P}[ e_3 ]) \\
            & = \min (\mathbf{p}_t, \mathbf{p}_f).
        \end{split}
    \end{equation}
\end{proof}

\paragraph{Proof of Theorem \ref{thm: prob2}}

\begin{proof}
    We denote the condition of $\Phi$ being satisfied as $\Phi = true$. Let event $\tilde e = \mathcal{A}_1 \implies \Phi$, there are two cases leading $\tilde e = true$: 1) $\mathcal{A}_1 = true \land \Phi = true$, and 2) $\mathcal{A}_1 = false$. 
    
    Since we have assumed $\tilde e =true$ in the theorem, the probability of $\Phi=true$ (without assumption $\mathcal{A}_1$) is at least equal to the probability of case 1) happens. Because $\Phi$ has to be true if case 1) happens, and $\Phi$ can be either true or false if case 2) happens. Additionally, the probability of case 1) happening only depends on $\mathcal{A}_1$. Hence we get $\mathbb[\Phi = true] \ge \mathbb{P}[\mathcal{A}_1 = true]$ for each proposition evaluation.
    
    From Theorem \ref{thm: prob} we know that $\mathbb{P}[\mathcal{A}_1 = true] \ge \min \left( \mathbf{p}_t, \mathbf{p}_f \right)$. Note that this probability is for a single proposition evaluation whose result is true or false. If the operation cycle contains at most $N_{max}$ proposition evaluations whose results are not \UNC{}, $\mathbb{P}[\mathcal{A}_1 = true] \ge \min \left( \mathbf{p}_t, \mathbf{p}_f \right)^{N_{max}}$ since all the evaluations are independent.

    Therefore, we get $\mathbb[\Phi = true] \ge \mathbb{P}[\mathcal{A}_1 = true]\ge \min \left( \mathbf{p}_t, \mathbf{p}_f \right)^{N_{max}}$.
\end{proof}

\section{Verification using NuSMV}
\lstinputlisting[language=NuSMV]{figures/verification/main.smv}
